# Supplementary material for: Egocentric Video-Language Pretraining
Source: arXiv:2206.01670 source file (2022-10-13)
Supplement: Supplementary file 1 [file 1_egoclip_filtering.tex]

\begin{figure}[h]
\centering
\vspace{-0.5cm}
\subfigure[The double-sized stereo video]{
\centering
\begin{minipage}[t]{0.45\textwidth}
\centering
\includegraphics[width=0.7\linewidth]{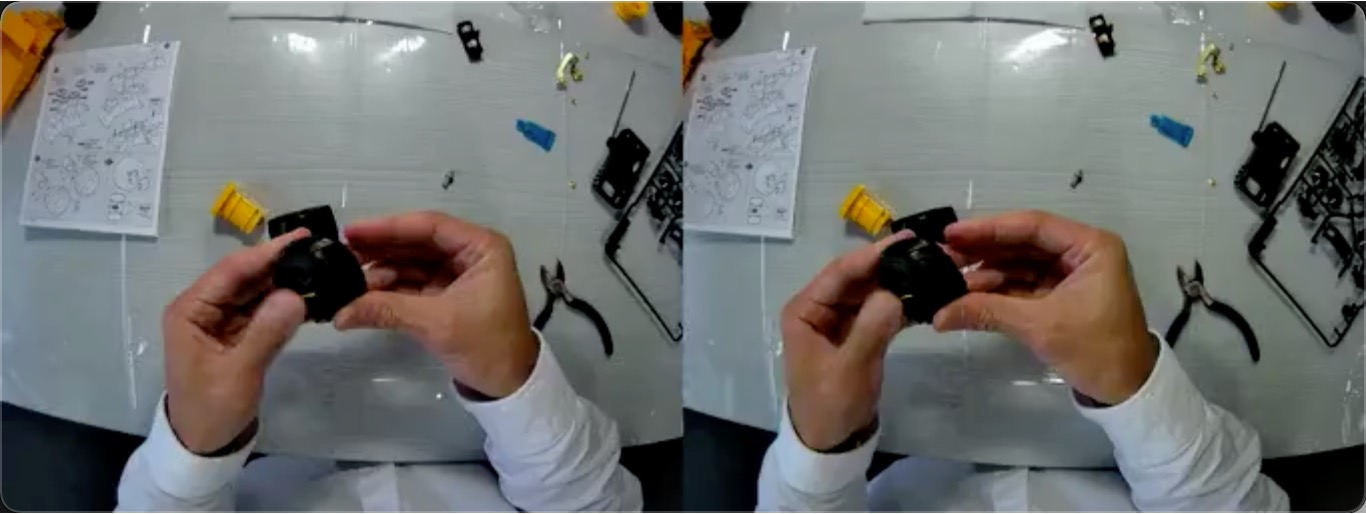}
\label{case_1}
\end{minipage}
}
\subfigure[The video with an undesired aspect ratio]{
\centering
\begin{minipage}[t]{0.45\textwidth}
\centering
\includegraphics[width=0.12\linewidth]{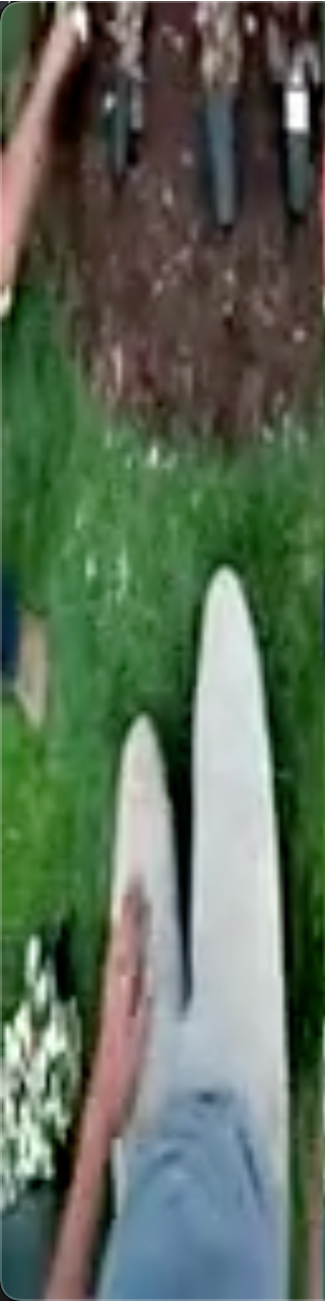}
\end{minipage}
}
\caption{Examples of noise videos}
\label{fig_egoclip_filtering}
\centering
\vspace{-0.5cm}
\end{figure}
